# Supplementary material for: Hierarchical clustering of bipartite data sets based on the statistical significance of coincidences
Source: arXiv:2004.14764 ancillary file (2020-07-24)
Supplement: Supplementary file 1 [file SM.pdf]

# Supplementary Material for "Hierarchical clustering of bipartite data sets based on the statistical significance of coincidences"

Ignacio Tamarit, María Pereda, and José A. Cuesta

## Supplementary figures

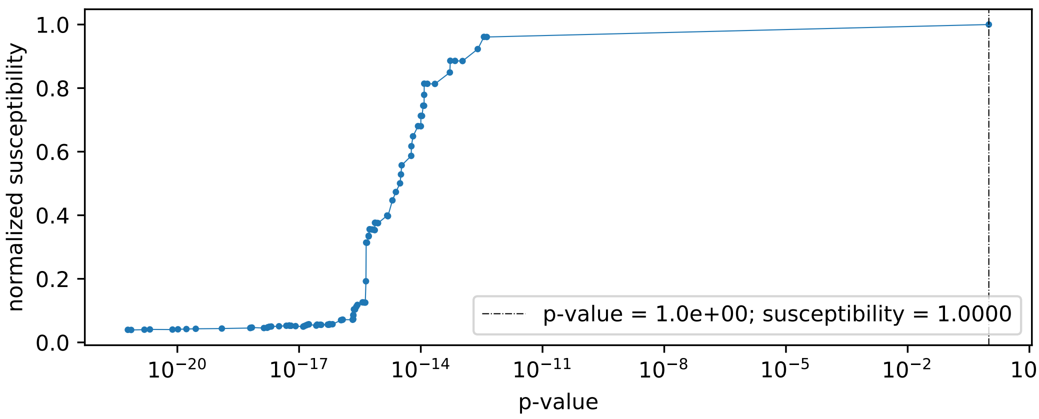


**Supplementary Figure S1:** Normalized susceptibility as a function of the thresholds where the dendrogram clusters split, of a two-cluster bipartite network. Dots are joined by lines as a aid to the eye.

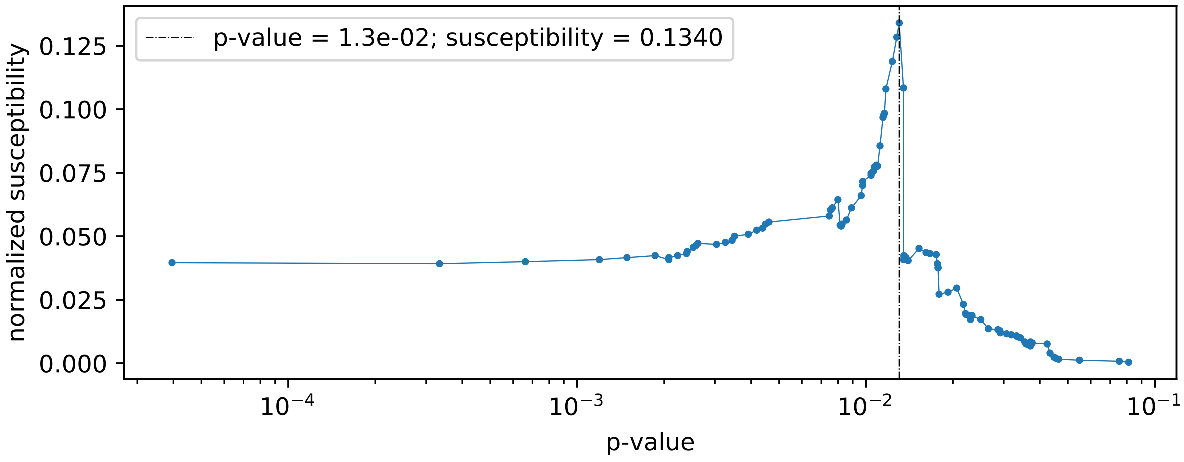


**Supplementary Figure S2:** Normalized susceptibility as a function of the thresholds where the dendrogram clusters split, of a random network. Normalized susceptibility values (dots) are joined by lines as a aid to the eye.

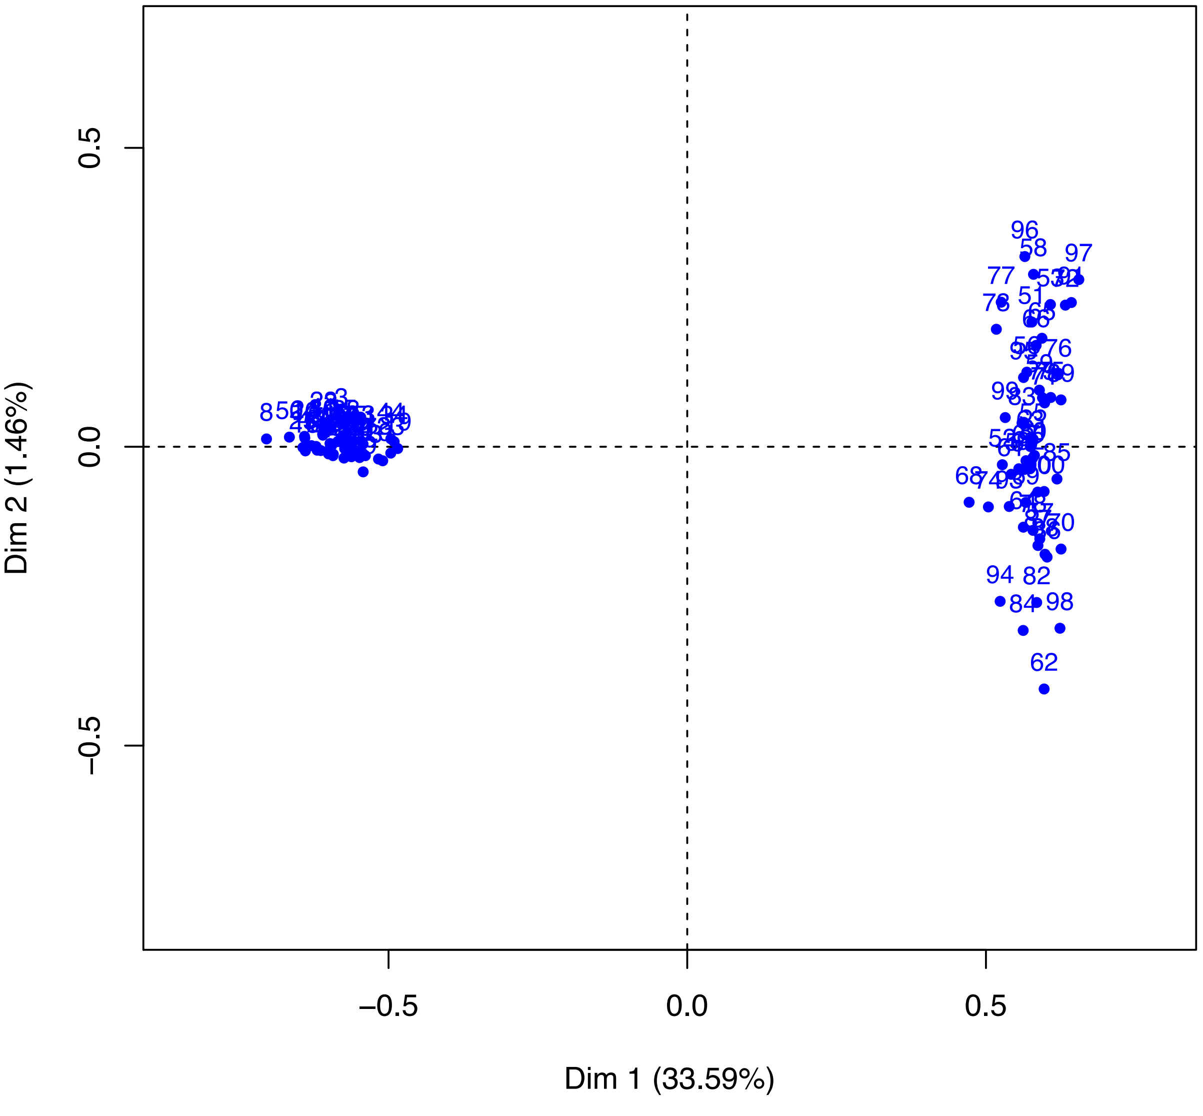


**Supplementary Figure S3:** Factors map of a two-cluster bipartite network.

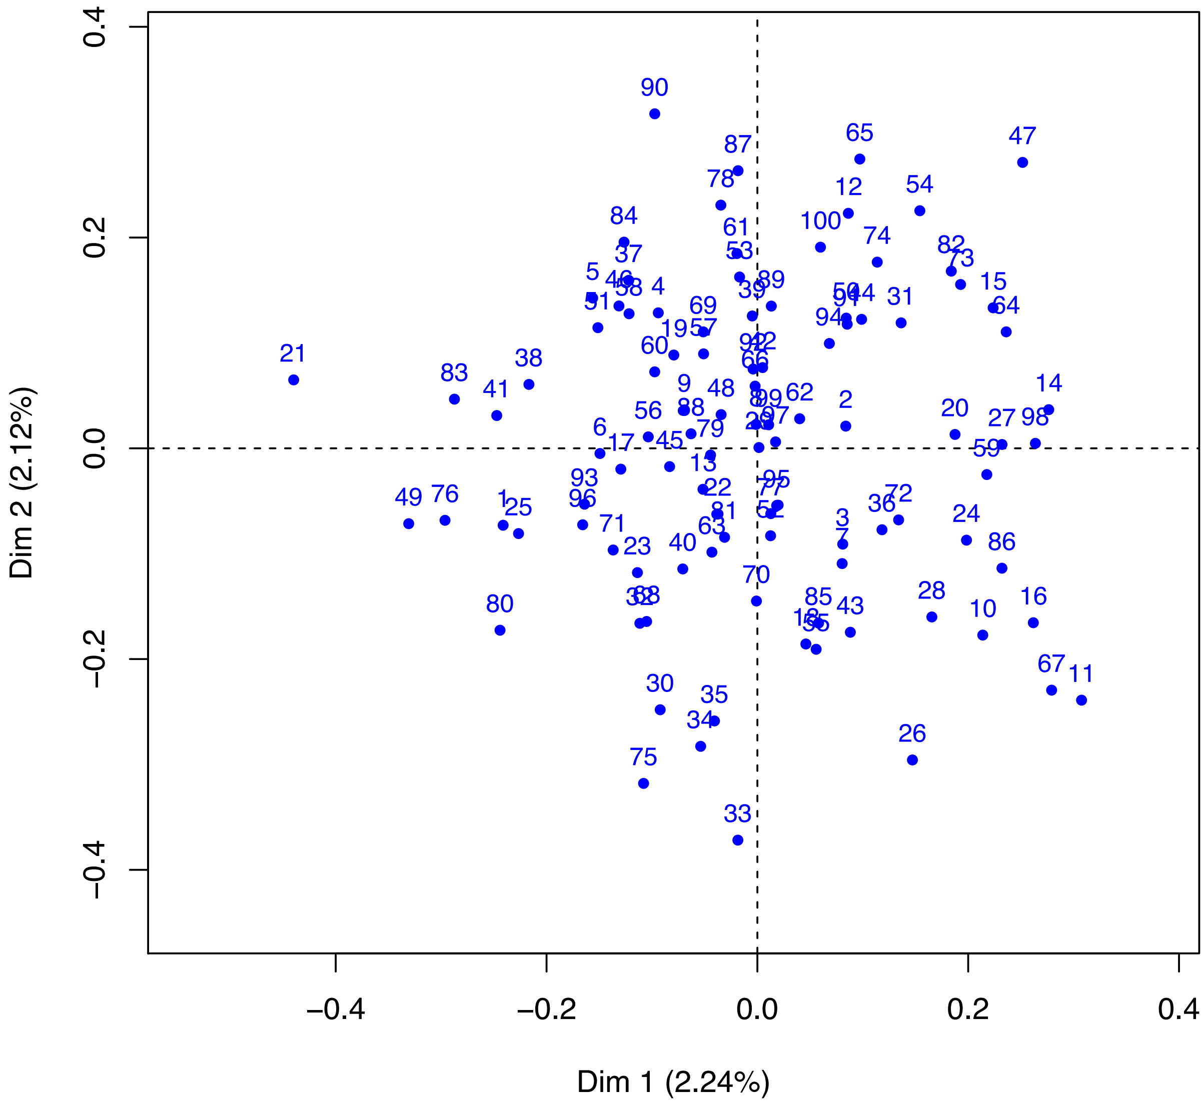


**Supplementary Figure S4:** Factors map of a random network.

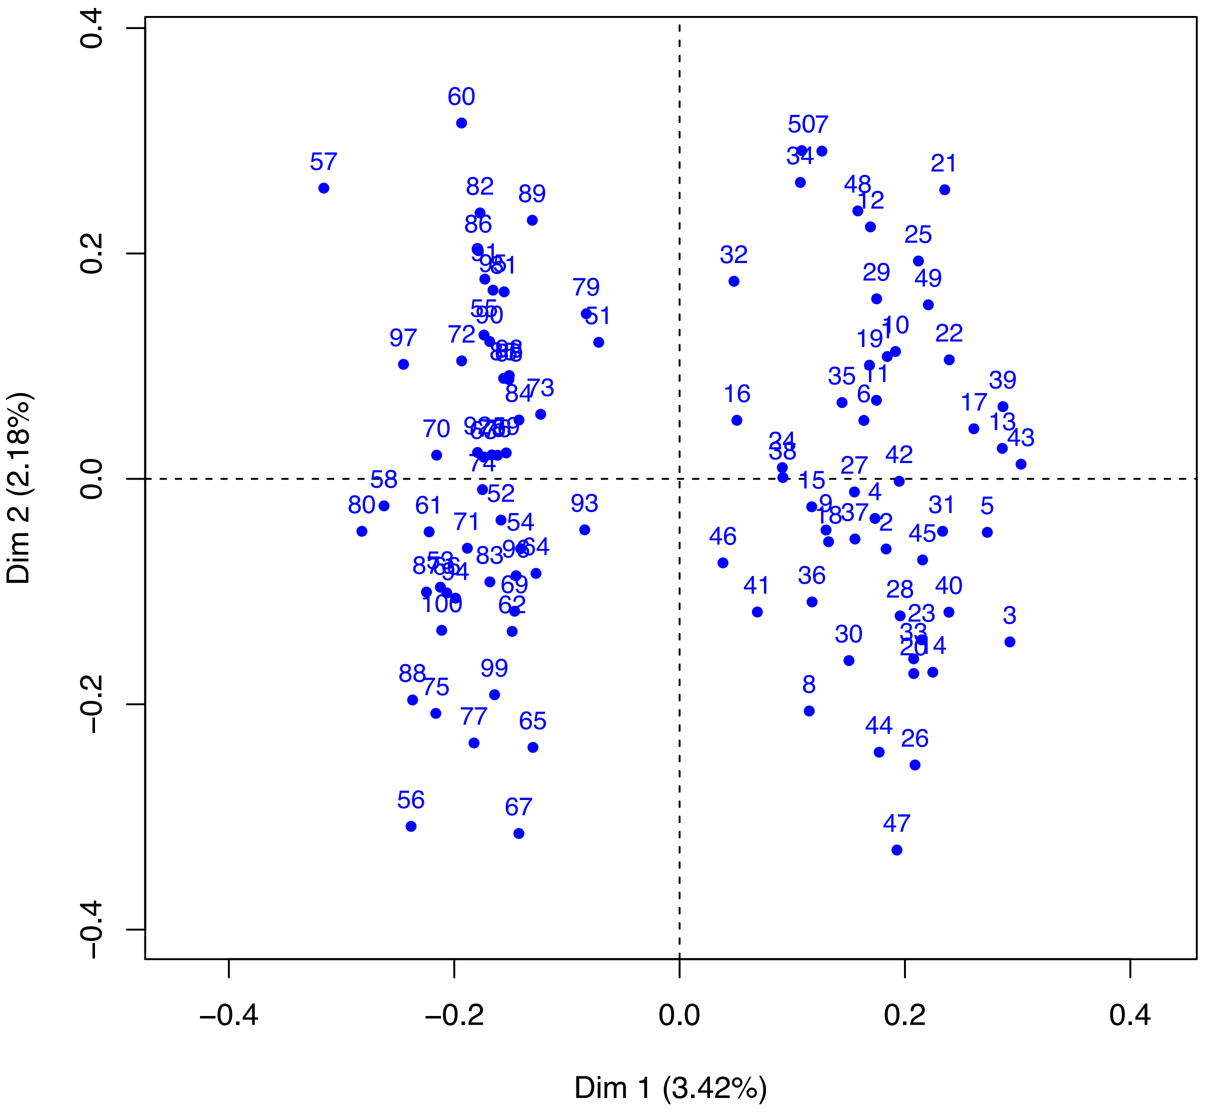


**Supplementary Figure S5:** Factors map of a a bipartite network with some clusters (*p_add*=0.35).

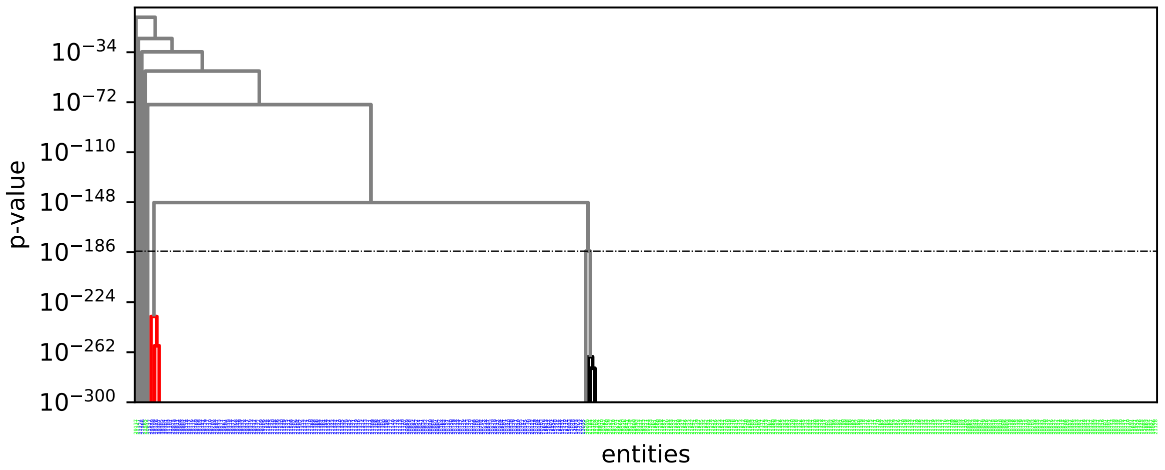


**Supplementary Figure S6:** Dendrogram of the clustering of roll cast votes of Congressmen for House 114. Colors in the dendrogram represent cluster of entities, except for grey representing entities with no assigned cluster. Labels in the horizontal axis represent Congressmen and labels' colors their political party. (The dendrogram is cut at $p$-values around $10^{-300}$ because below this value the computation yielded underflows.)

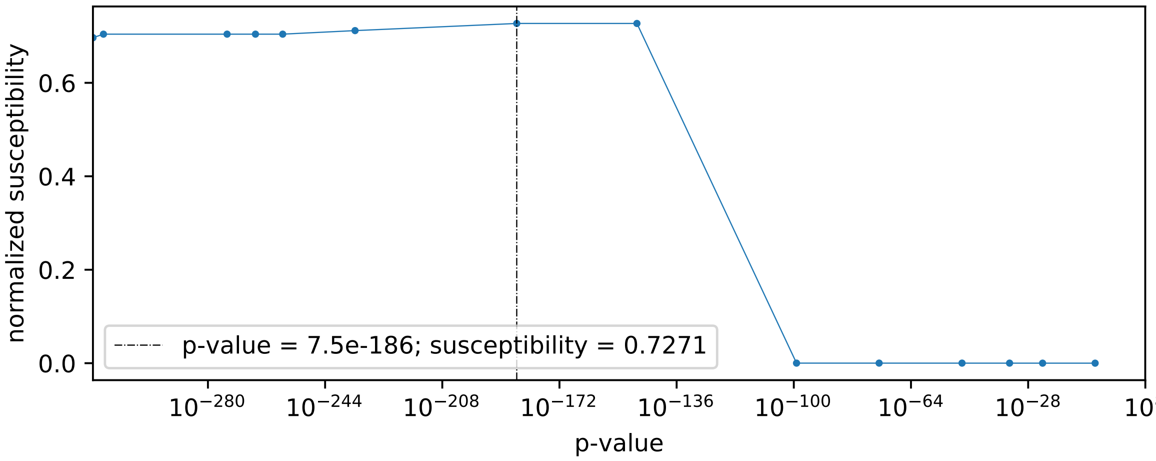


**Supplementary Figure S7:** Normalized susceptibility as a function of the thresholds where the dendrogram clusters split, for roll cast votes of Congressmen for House 114. Normalized susceptibility values (dots) are joined by lines as a aid to the eye.

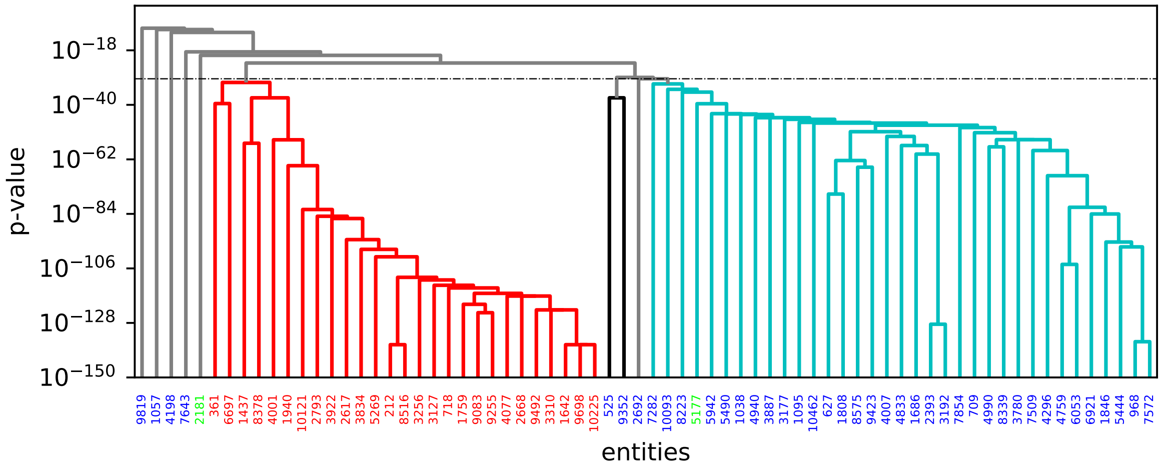


**Supplementary Figure S8:** Dendrogram of the clustering of roll cast votes of Congressmen for Senate 36. Colors in the dendrogram represent cluster of entities, except for grey representing entities with no assigned cluster. Labels in the horizontal axis represent Congressmen and labels' colors their political party.

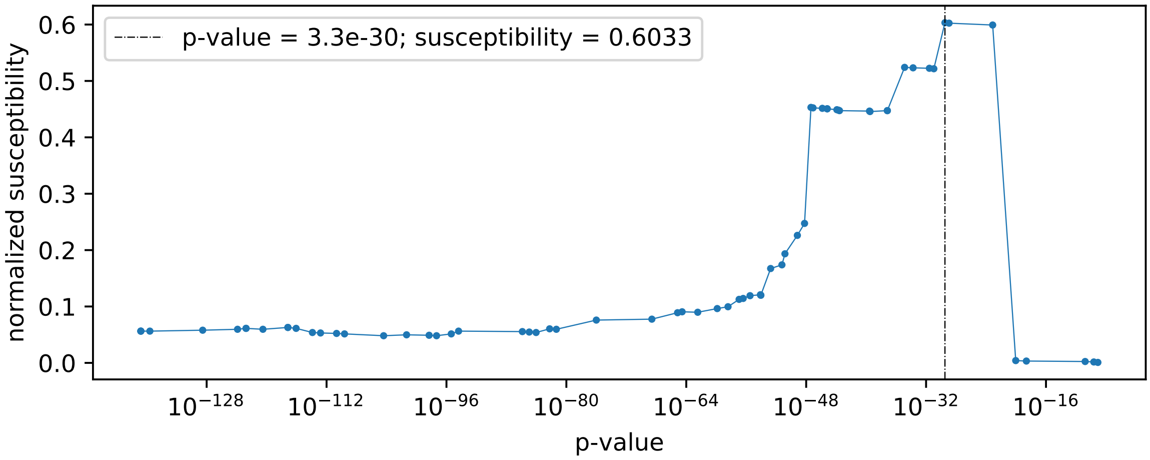


**Supplementary Figure S9:** Normalized susceptibility as a function of the thresholds where the dendrogram clusters split, for roll cast votes of Congressmen for Senate 36. Normalized susceptibility values (dots) are joined by lines as a aid to the eye.

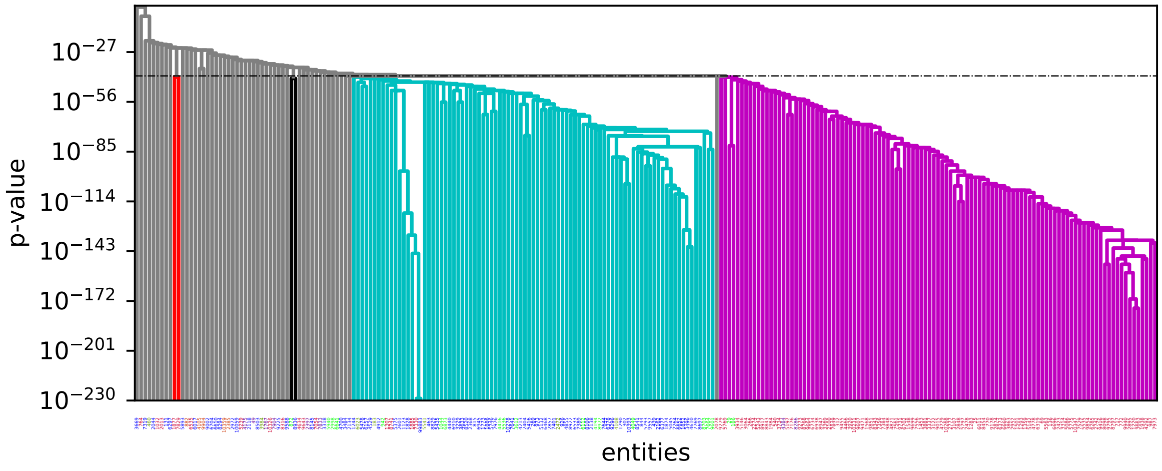


**Supplementary Figure S10:** Dendrogram of the clustering of roll cast votes of Congressmen for House 36. Colors in the dendrogram represent cluster of entities, except for grey representing entities with no assigned cluster. Labels in the horizontal axis represent Congressmen and labels' colors their political party.

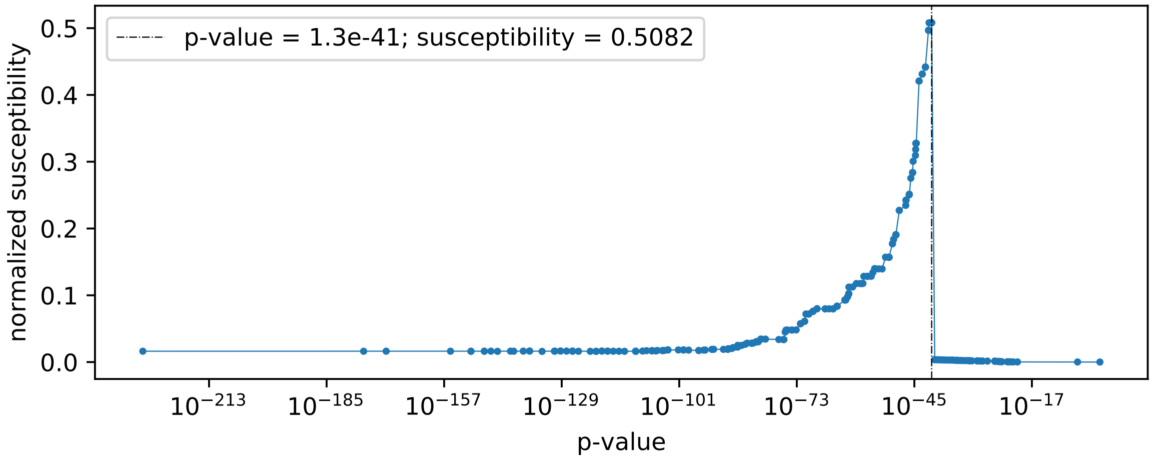


**Supplementary Figure S11:** Normalized susceptibility as a function of the thresholds where the dendrogram clusters split, for roll cast votes of Congressmen for House 36. Normalized susceptibility values (dots) are joined by lines as a aid to the eye.

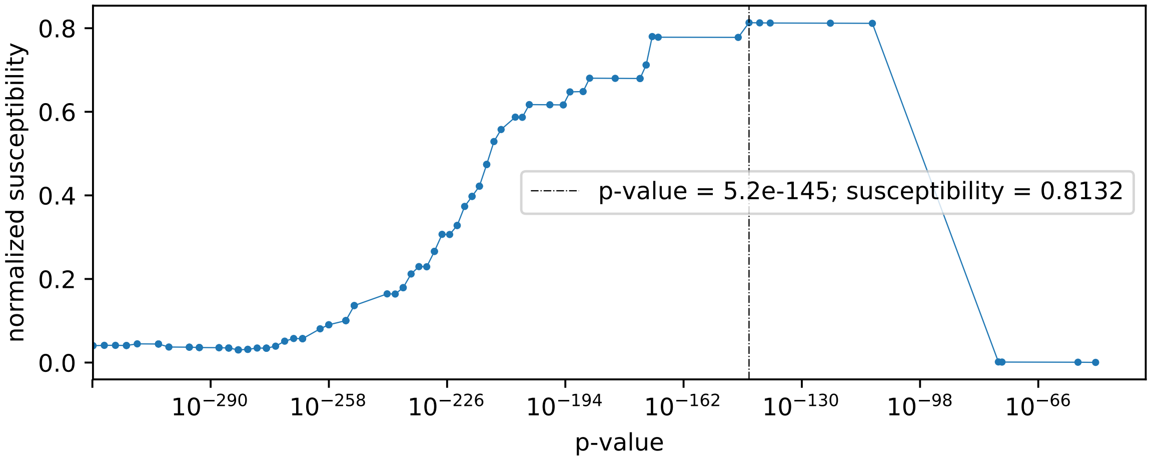


**Supplementary Figure S12:** Normalized susceptibility as a function of the thresholds where the dendrogram clusters split, for roll cast votes of Congressmen for Senate 114. Normalized susceptibility values (dots) are joined by lines as a aid to the eye.

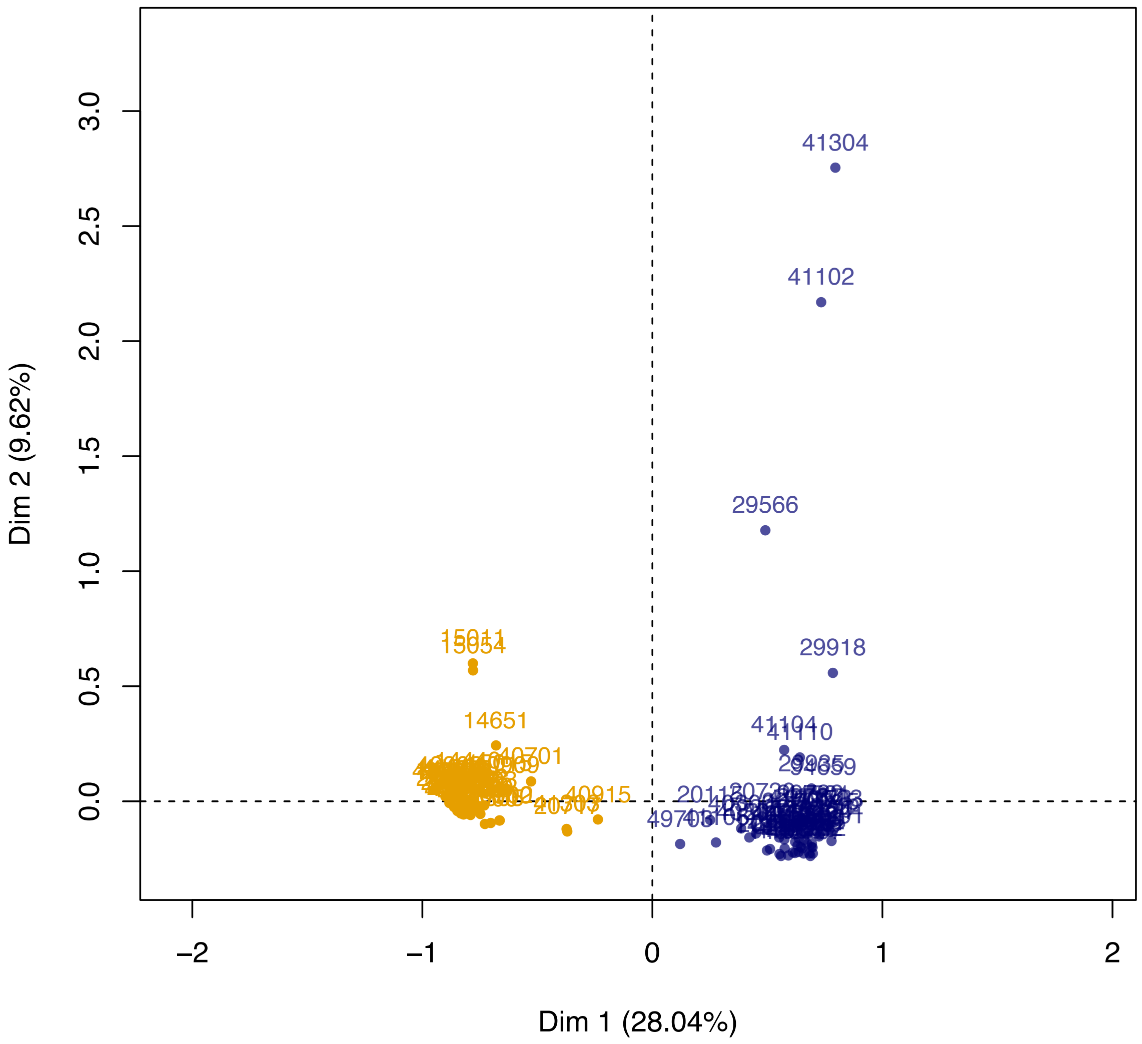


**Supplementary Figure S13:** Factors map of Congressmen for Senate 114. In colours, the party membership of the Congressmen.

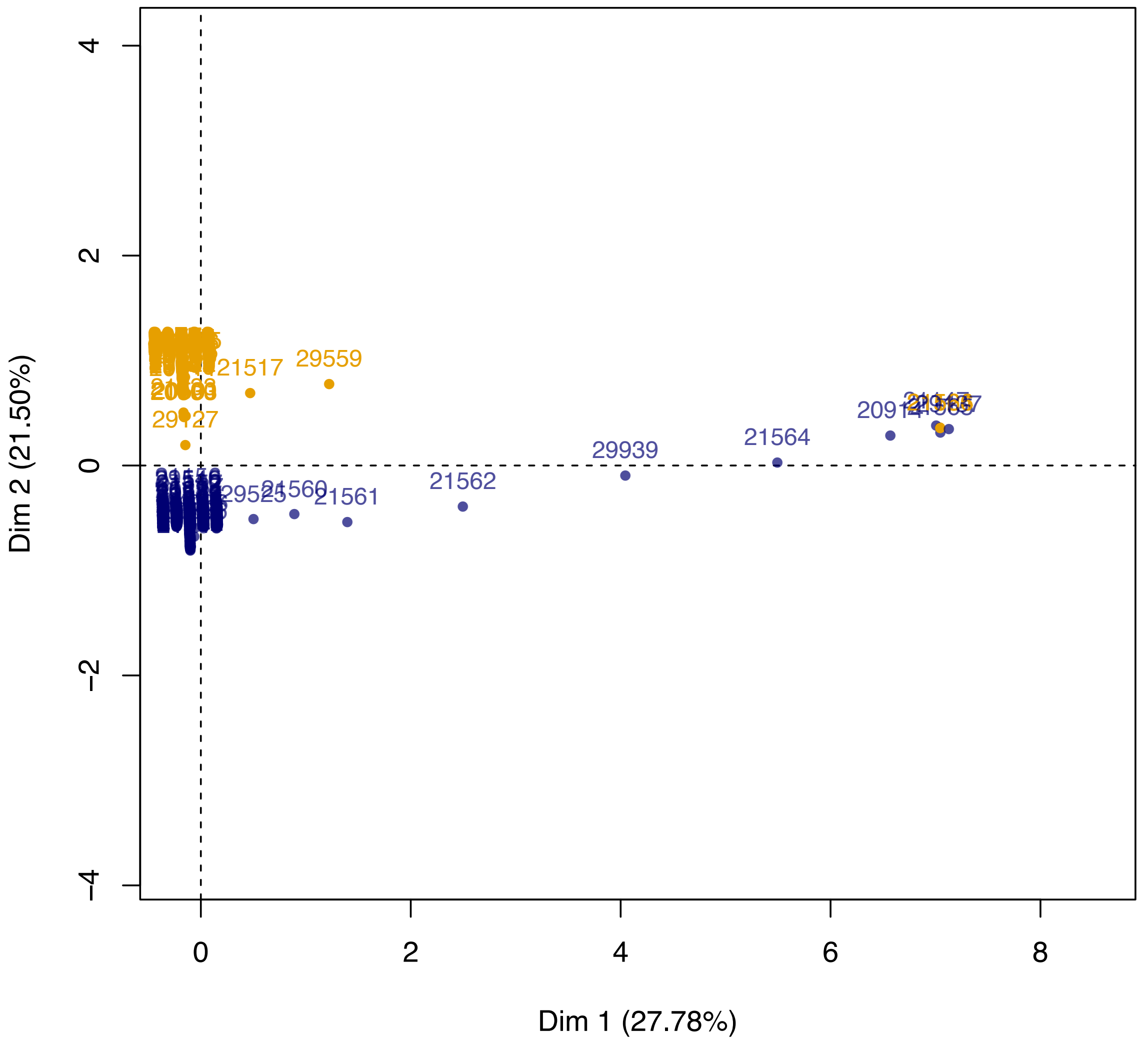


**Supplementary Figure S14:** Factors map of Congressmen for House 114. In colours, the party membership of the Congressmen.

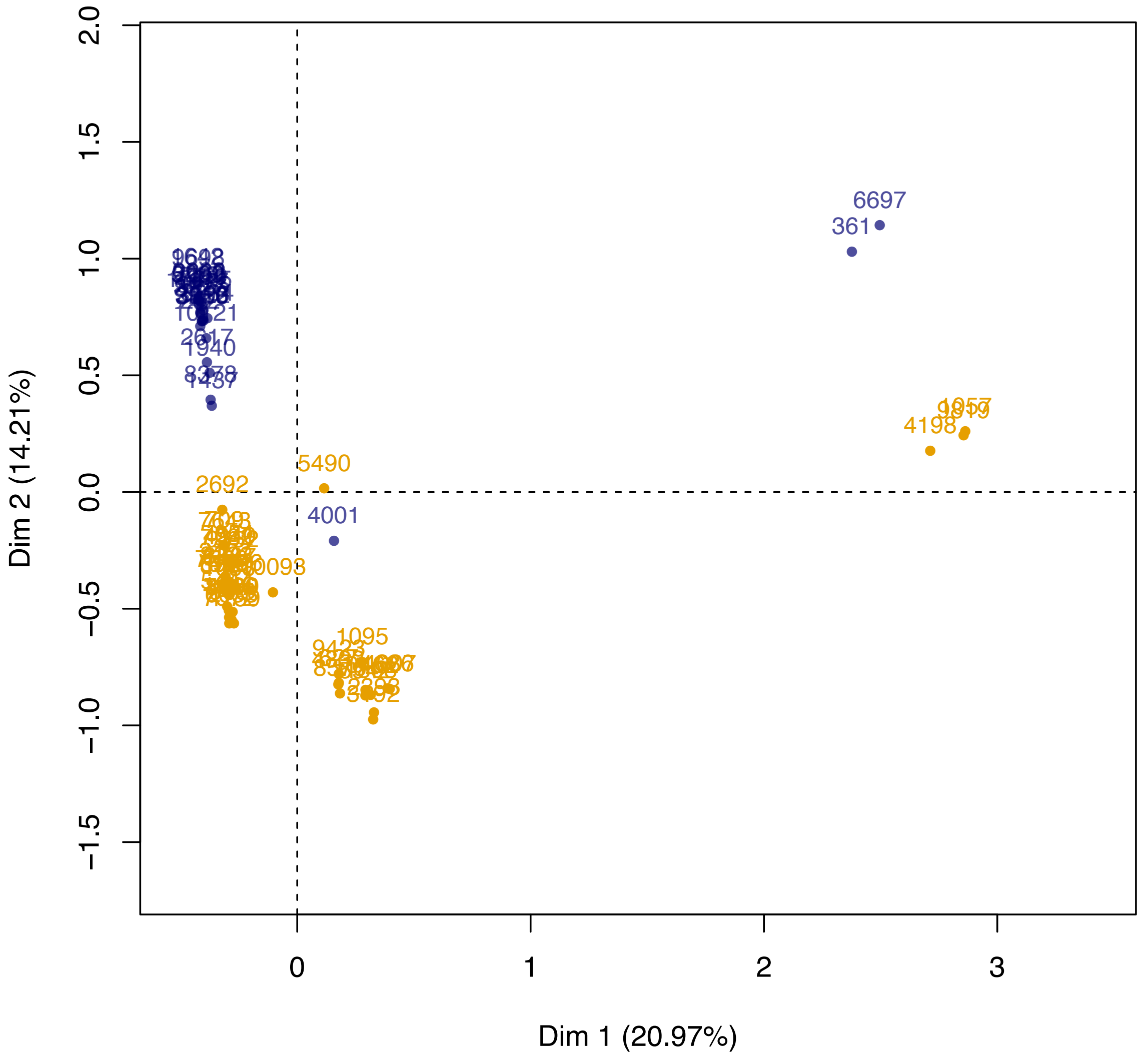


**Supplementary Figure S15:** Factors map of Congressmen for Senate 36. In colours, the party membership of the Congressmen.

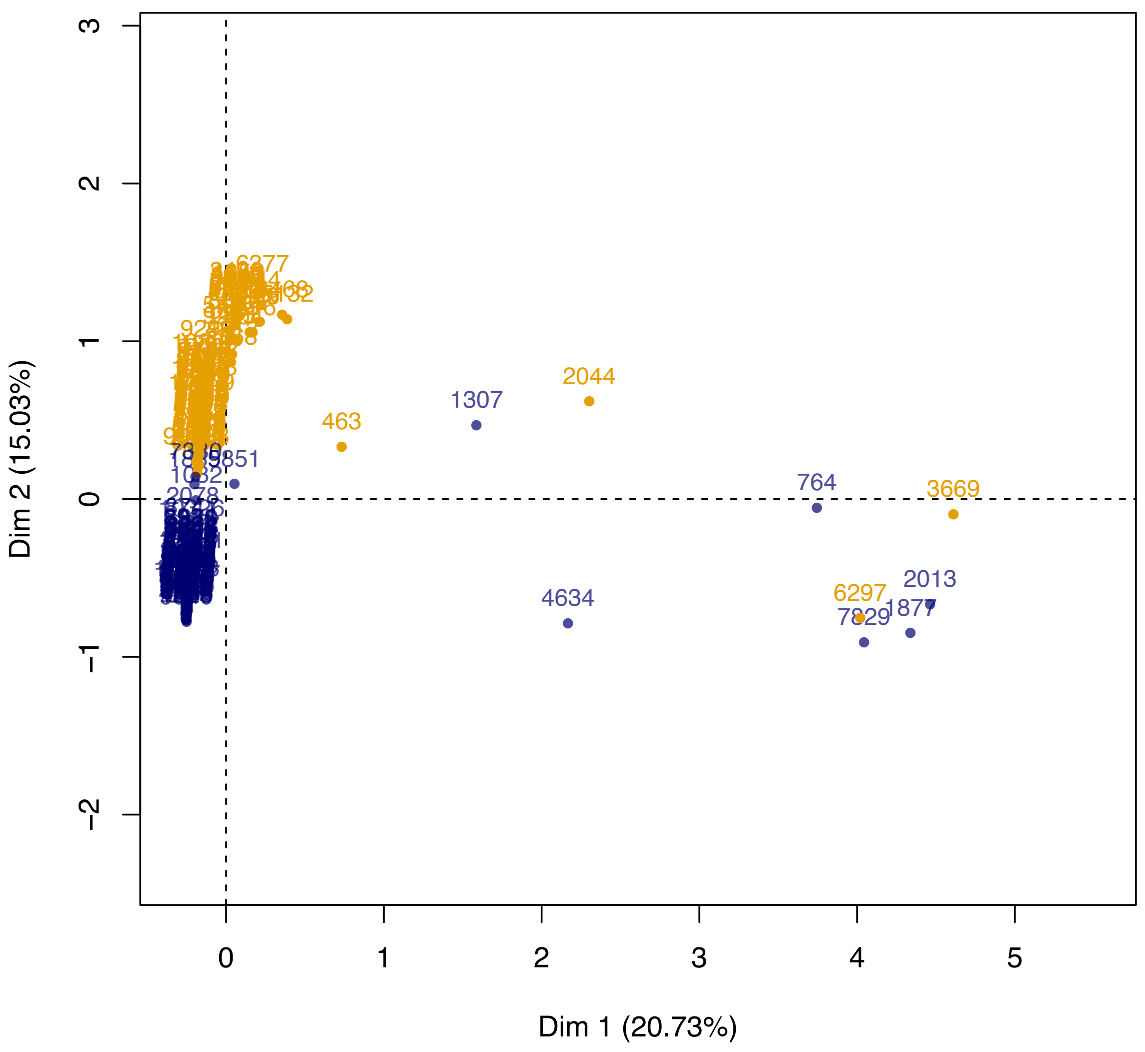


**Supplementary Figure S16:** Factors map of Congressmen for House 36. In colours, the party membership of the Congressmen.

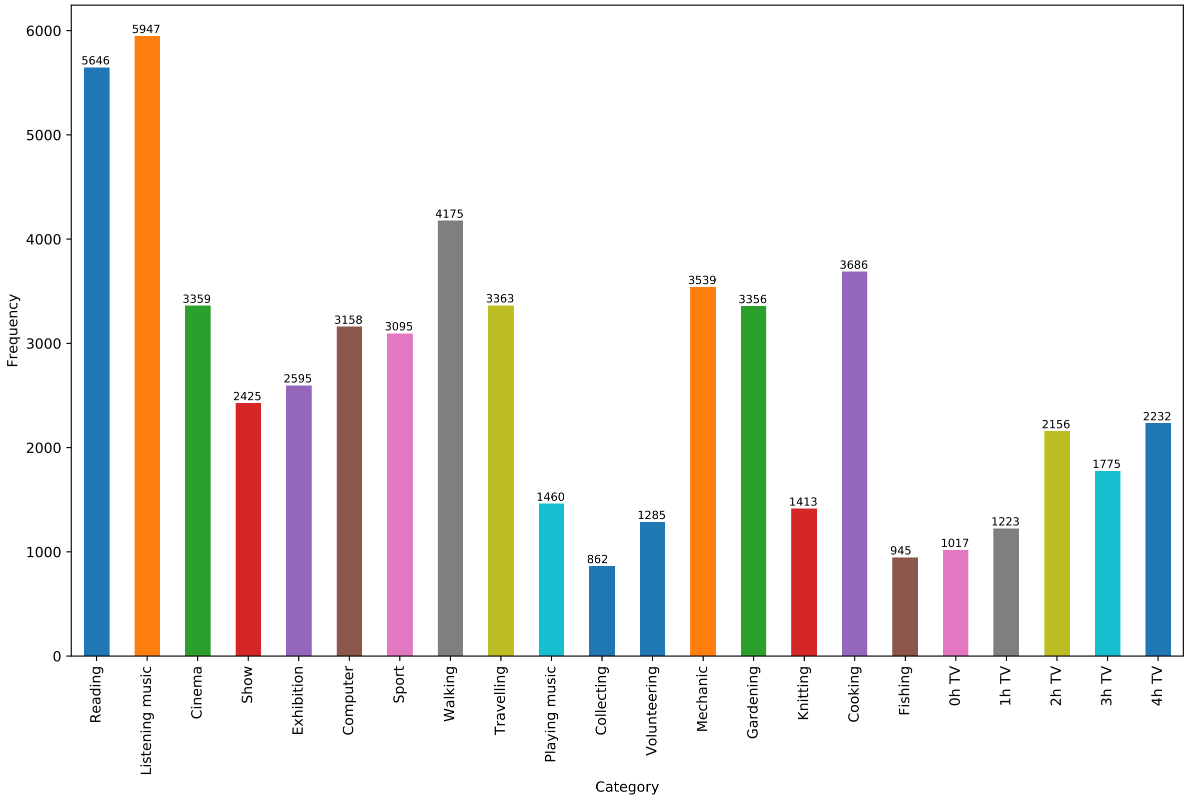


**Supplementary Figure S17:** Distribution of people' answers to the leisure activities in the hobbies dataset.

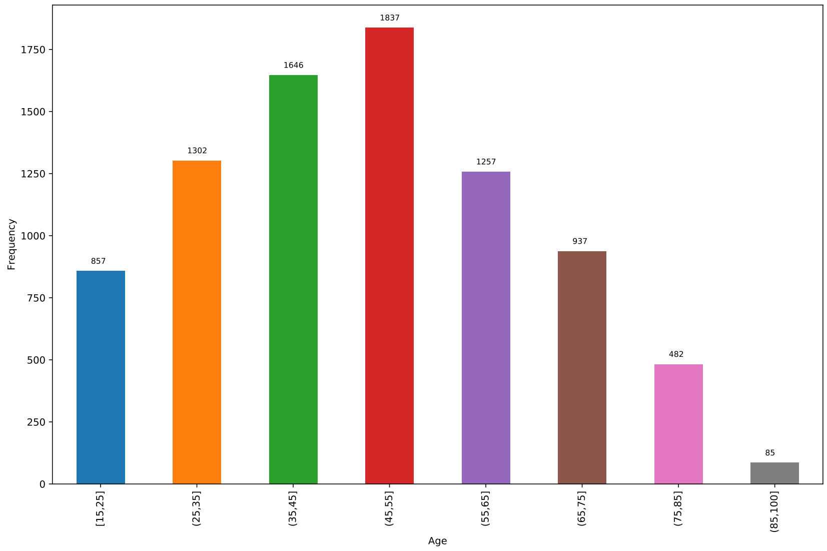


**Supplementary Figure S18:** Distribution of people' age to the leisure activities in the hobbies dataset.

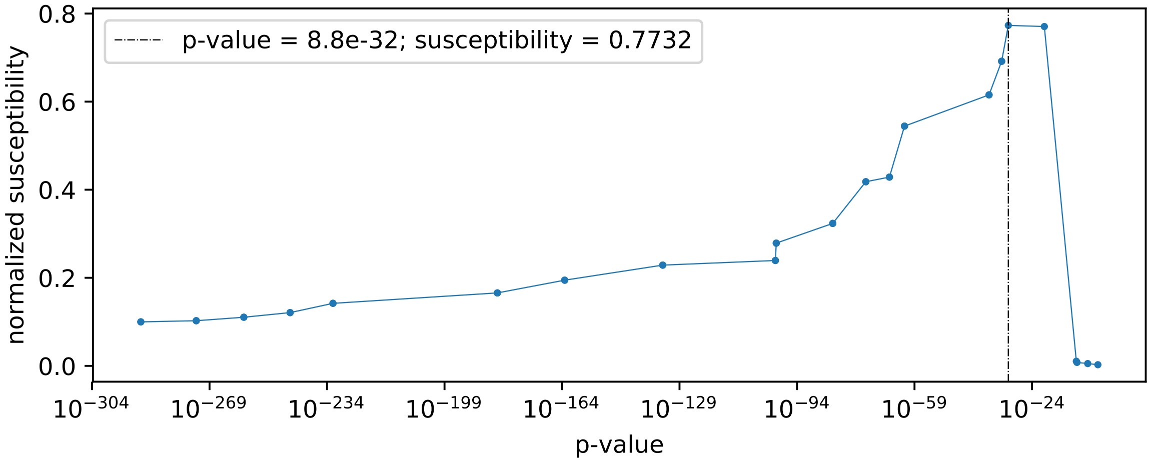


**Supplementary Figure S19:** Normalized susceptibility as a function of the thresholds where the dendrogram clusters split, for the leisure activities in the hobbies dataset. Normalized susceptibility values (dots) are joined by lines as a aid to the eye.

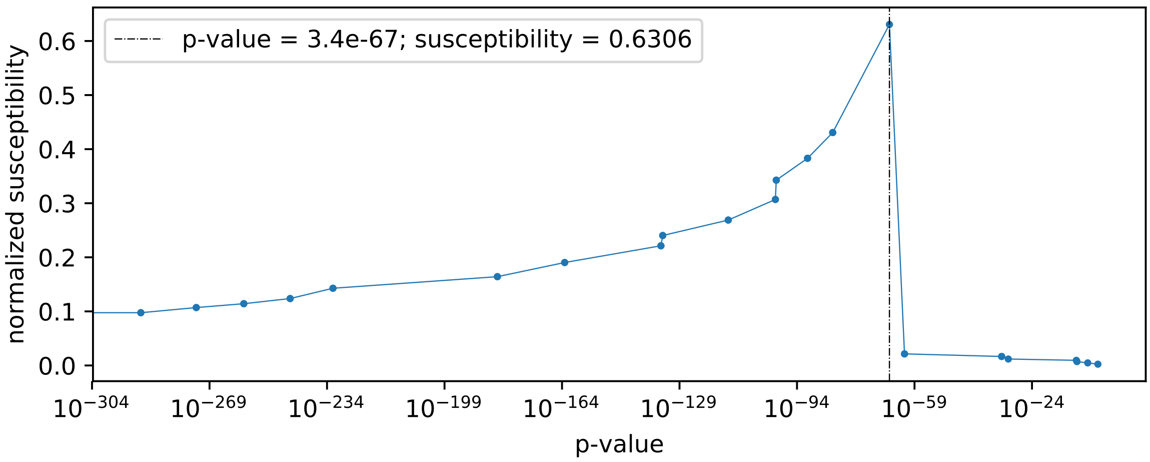


**Supplementary Figure S20:** Normalized susceptibility as a function of the thresholds where the dendrogram clusters split, for the leisure activities in the hobbies dataset, including sex as a feature. Normalized susceptibility values (dots) are joined by lines as a aid to the eye.

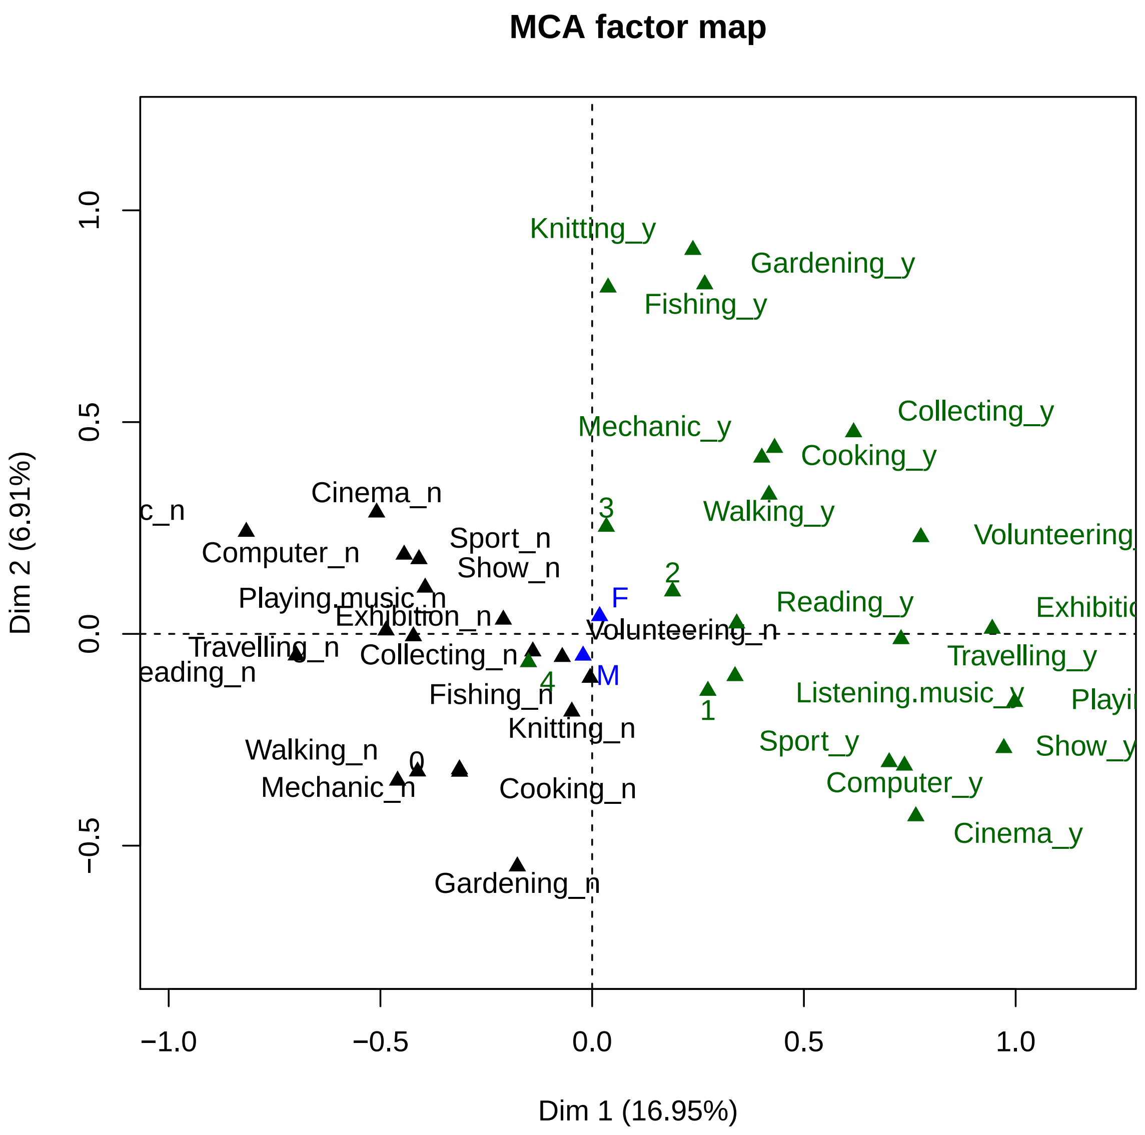


**Supplementary Figure S21:** Factors map of the hobbies data set, including sex as a feature. In green, the activity is performed; in black, the activity is not performed; in blue, the feature sex (F:female, M:male).

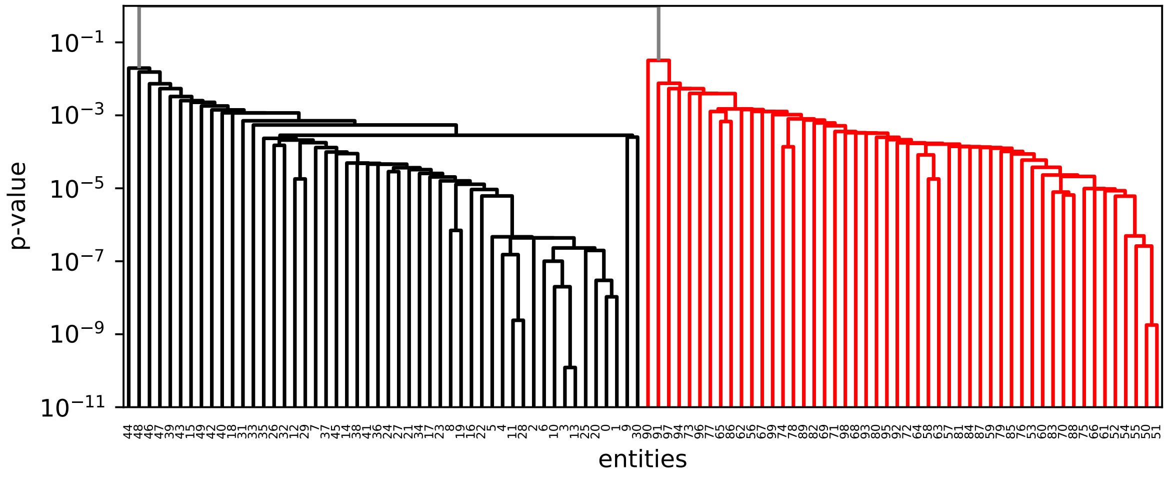


**Supplementary Figure S22:** Dendrogram of a two-cluster bipartite network, with heterogeneous degree distribution. The dashed line marks the point with highest susceptibility—that where the 'optimal' partition should be found.

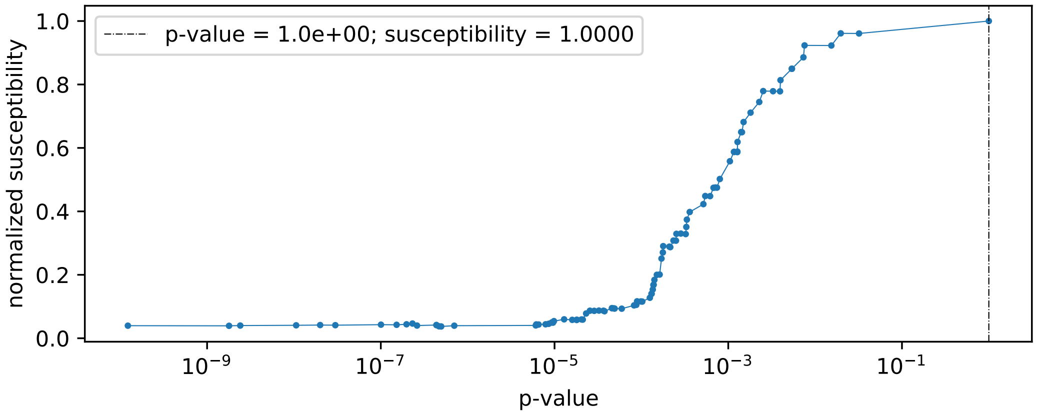


**Supplementary Figure S23:** Normalized susceptibility as a function of the thresholds where the dendrogram clusters split, of a two-cluster bipartite network with heterogeneous degree distribution. Dots are joined by lines as a aid to the eye.

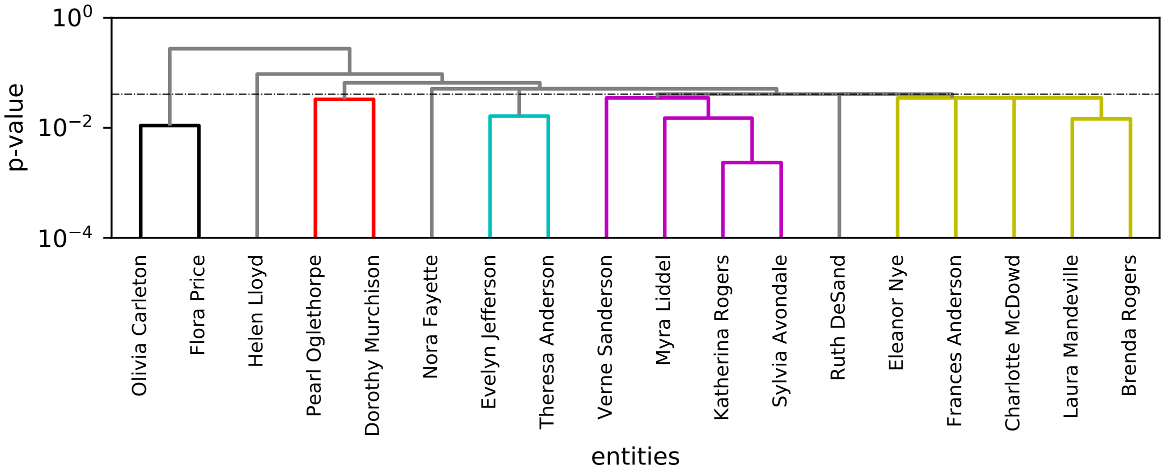


**Supplementary Figure S24:** Dendrogram of the clustering of women of the Southern Women dataset. The dashed line marks the point with highest susceptibility—that where the 'optimal' partition should be found. ClusterBip found 3 women whose attendance to events behavior is different from the rest (Helen, Nora, and Ruth); and five clusters. We see a cluster with Olivia and Flora, which are the most separated in the second group of the original paper [49] and part of the blue group in ref [25]. Helen and Nora do not have a similar pattern to anyone else (they are also somewhat separated in the second group [49]). In the original paper, Pearl and Dorothy do not appear in the figures; in ref. [25] they belong to the blue cluster but they have links with the red cluster. Evelyn and Theresa go to similar events, they also appear close to each other in the results of ref [25]. Verne, Myna, Katherine and Sylvia form their own cluster, which is the left half of second group in the original paper, and part of the blue group in ref [25]. Ruth is classified apart since she attended an event (E9) that was mainly attended by members of the second group [49]. Finally we have Eleanor, Frances, Charlotte, Laura and Brenda's group.

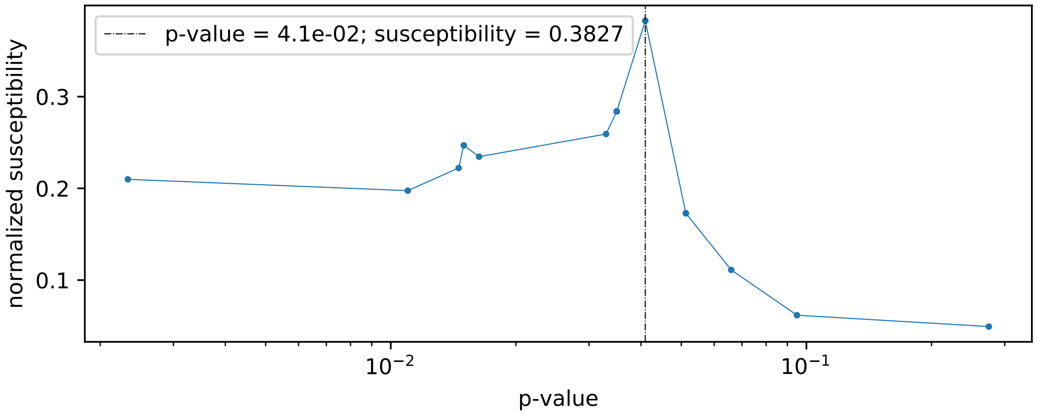


**Supplementary Figure S25:** Normalized susceptibility as a function of the thresholds where the dendrogram clusters split, for the clustering of women of the Southern Women dataset. Dot are joined by lines as a aid to the eye.

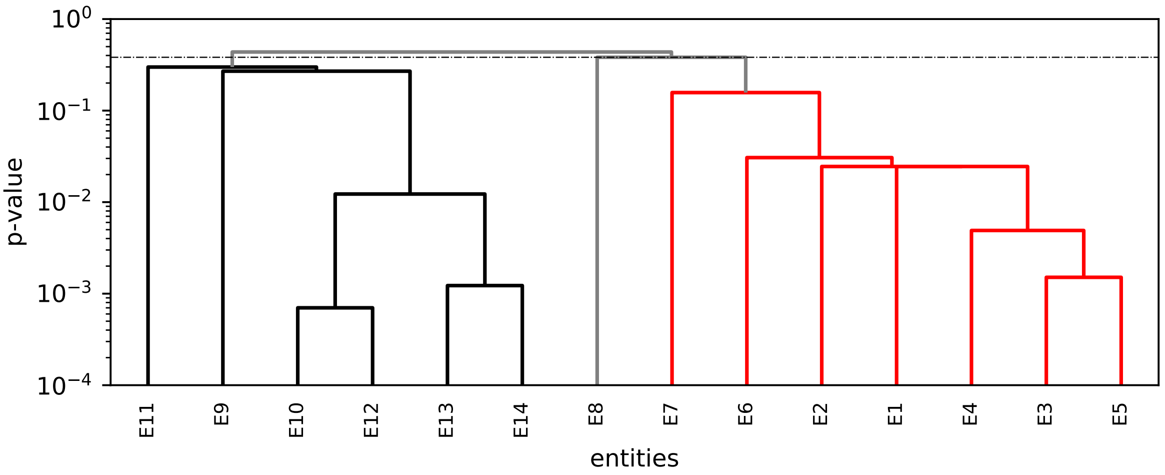


**Supplementary Figure S26:** Dendrogram of the clustering of events of the Southern Women dataset. The dashed line marks the point with highest susceptibility—that where the 'optimal' partition should be found. ClusterBip found the same groups as in ref. [25], except for the event $E8$ that is not classified in any cluster, maybe because it is an event attended by women from all groups that seems to be a popular event.

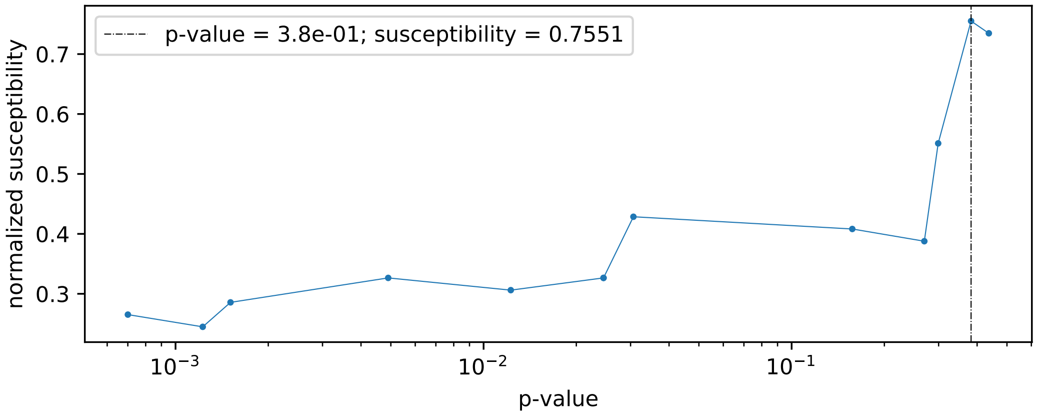


**Supplementary Figure S27:** Normalized susceptibility as a function of the thresholds where the dendrogram clusters split, for the clustering of events of the Southern Women dataset. Dot are joined by lines as a aid to the eye.
